# Supplementary material for: Electronic excited states in extreme limits via ensemble density functionals
Source: arXiv:2205.07136 source file (2022-10-15)
Supplement: Supplementary file 1 [file Supp-Resubmit-Final.pdf]

# Supplementary Material for "Electronic excited states in extreme limits via ensemble density functionals"

Tim Gould

*Queensland Micro- and Nanotechnology Centre,*

*Griffith University, Nathan, Qld 4111, Australia**

Derk P. Kooi and Paola Gori-Giorgi

*Department of Chemistry & Pharmaceutical Sciences and*

*Amsterdam Institute of Molecular and Life Sciences (AIMMS),*

*Faculty of Science, Vrije Universiteit, De Boelelaan 1083,*

*1081HV Amsterdam, The Netherlands*

Stefano Pittalis

*CNR-Istituto Nanoscienze, Via Campi 213A, I-41125 Modena, Italy*

## TABLE OF CONTENTS

Supplementary material for "Electronic excited states in extreme limits via ensemble density functionals". Contains the following sections:

I. A detailed proof of key results from the paper

II. Details of Harmonium atoms and their behaviours

III. Details of scaling to low densities

IV. Technical details for the excited state calculations reported in the paper

## I. PROOF OF KEY RESULTS

Before beginning the proof, let us stress key notation. Quantities with a "hat" on top are operators, with $\hat{V}_{ee}$ the electron-electron Coulomb repulsion operator, $\hat{T}$ the electronic kinetic energy operator, $\hat{n}$ the density operator, and $\hat{v}_{\text{label}} := \int v_{\text{label}}(\boldsymbol{r})\hat{n}(\boldsymbol{r})d\boldsymbol{r}$ a potential operator. Lowercase vectors, $\boldsymbol{v}$ are in three dimensions, while uppercase vectors, $\boldsymbol{V}$, collect vector information for many electrons or coordinates. Thus, e.g., $P_N(\boldsymbol{R}) = P_N(\boldsymbol{r}_1, \boldsymbol{r}_2, \cdots \boldsymbol{r}_N)$ represent the same distribution.

We sometimes use (improperly) the term 'wavefunction' to indicate minimizers that are actually distributions. This does not pose any problem (except for the improper naming), since the mathematical subtleties concerning the enlargment of the space from wavefunctions to probability densities are now well established in the ground-state SCE case [1, 2], and they directly apply also here.

Lagrangians feature throughout the discussion, and take the form $L[a, b, c; x, y, z]$ where variables before the semicolon are constraints and variables after the semicolon are to be minimized over.

We differ from the main text in one important way. Rather than using the short-hand $\mathcal{E}^{\boldsymbol{w}}[n]$ for an ensemble quantity with given weights, $\boldsymbol{w}$, we often write $E[n, \{w_P\}]$ to maintain clear and consistent notation throughout the proof. Where key results are presented, we use both notations.

* t.gould@griffith.edu.au

### A. Equivalence of ensembles and pure state for the SCE functional

To begin the proof, we first show that the ground-state Strictly-Correlated Electrons (SCE) functional can be equivalently seen as having a pure state as minimizer or an ensemble with weights that can be chosen arbitrarily [1]. The ground state SCE functional is defined as,

$$V_{\mathrm{ee}}^{\mathrm{SCE}}[n] := \min_{\Psi\to n} \langle\Psi|\hat{V}_{ee}|\Psi\rangle \ . \tag{S1}$$

For present purposes, the minimizer here can be seen as a wavefunction $\Psi$ (although, strictly speaking we should not call it a wavefunction since it has infinite kinetic energy – see Ref. 3 for a mathematical rigorous statement) that has a corresponding probability distribution $|\Psi(\boldsymbol{r}_1,\boldsymbol{r}_2,\dots\boldsymbol{r}_N)|^2 = P_N(\boldsymbol{r}_1,\boldsymbol{r}_2,\dots\boldsymbol{r}_N) \geq 0$, where $P_N$ arises from the minimization,

$$V_{\mathrm{ee}}^{\mathrm{SCE}}[n] = \min_{P_N\to n} \int d\boldsymbol{r}_1 d\boldsymbol{r}_2\cdots d\boldsymbol{r}_N P_N(\boldsymbol{r}_1,\boldsymbol{r}_2,\dots\boldsymbol{r}_N)\sum_{p<q}\frac{1}{|\boldsymbol{r}_p-\boldsymbol{r}_q|}. \tag{S2}$$

Here, $P_N \to n$ means $N\int d\boldsymbol{r}_2 d\boldsymbol{r}_3\cdots d\boldsymbol{r}_N P_N(\boldsymbol{r},\boldsymbol{r}_2,\dots\boldsymbol{r}_N) = n$.

The corresponding Lagrangian is,

$$\begin{aligned} L_{\mathrm{SCE}}[n; v_{\mathrm{SCE}},\mu] = &\int d\boldsymbol{r}_1 d\boldsymbol{r}_2 \dots d\boldsymbol{r}_N P_N(\boldsymbol{r}_1,\boldsymbol{r}_2,\dots\boldsymbol{r}_N) \\ &\times\left(\sum_{p<q}\frac{1}{|\boldsymbol{r}_p-\boldsymbol{r}_q|}+\sum_p v_{\mathrm{SCE}}(\boldsymbol{r}_p)-\mu(\boldsymbol{r}_1,\boldsymbol{r}_2,\dots\boldsymbol{r}_N)\right) \\ &-\int d\boldsymbol{r} n(\boldsymbol{r}) v_{\mathrm{SCE}}(\boldsymbol{r}), \end{aligned} \tag{S3}$$

where $v_{\mathrm{SCE}}(\boldsymbol{r})$ is the SCE potential, the Lagrange multiplier for the density constraint, and $\mu(\boldsymbol{r}_1,\boldsymbol{r}_2,\dots\boldsymbol{r}_N) \geq 0$ is the Karush-Kuhn-Tucker multiplier for the positivity of the probability distribution $P_N$. $\Psi$ can then be constructed by taking the square root of $P_N$ and inserting spin and the appropriate anti-symmetry.

We could have also performed our minimization by instead searching over all ensembles with *arbitrary* weights $\{\hat{\Gamma}\}$,

$$V_{\mathrm{ee}}^{\mathrm{SCE}}[n] := \min_{\hat{\Gamma}\to n} \mathrm{Tr}[\hat{\Gamma}\hat{V}_{ee}]. \tag{S4}$$

In principle, since we enlarge the space over which we search, we can only obtain a result that is below or equal to that of equation S1, but we will show that we obtain exactly the same result, whether we optimize over the weights or whether we fix them, as in EDFT (see

Sec. I A 1). Now, the corresponding Lagrangian is,

$$\begin{aligned} L_{\mathrm{SCE}}[n;\{w_P\},\{\Psi_P\},v_{\mathrm{SCE}},\{\mu_P\},\{\epsilon_{PQ}\}] = & \sum_P w_P \langle \Psi_P|\hat{V}_{ee}|\Psi_P\rangle \\ & + \int d\boldsymbol{r} v_{\mathrm{SCE}}(\boldsymbol{r}) \left( \sum_P w_P \langle \Psi_P|\hat{n}(\boldsymbol{r})|\Psi_P\rangle - n(\boldsymbol{r}) \right) \\ & - \sum_{PQ} \epsilon_{PQ}(\langle \Psi_P|\Psi_Q\rangle - \delta_{PQ}) - \sum_P \mu_P w_P \ , \end{aligned} \tag{S5}$$

where we expanded $\hat{\Gamma} = \sum_P w_P|\Psi_P\rangle\langle\Psi_P|$ in terms of its eigenvalues (weights) $\{w_P\}$ and eigenstates $\{|\Psi_P\rangle\}$. Here, $\{\mu_P\}$ are the Karush-Kuhn-Tucker multipliers for the positivity of the weights and $\{\epsilon_{PQ}\}$ are the Lagrange multipliers for the orthonormality of the eigenstates $\{|\Psi_P\rangle\}$.

Taking the derivative to $\langle\Psi_P|$ we obtain the primal optimality condition,

$$w_P\hat{V}_{ee}|\Psi_P\rangle + w_P\hat{v}_{\mathrm{SCE}}|\Psi_P\rangle = \sum_Q \epsilon_{PQ}|\Psi_Q\rangle, \tag{S6}$$

where we have defined,

$$\hat{v}_{\mathrm{SCE}} := \int d\boldsymbol{r} v_{\mathrm{SCE}}(\boldsymbol{r})\hat{n}(\boldsymbol{r}). \tag{S7}$$

Both $\hat{V}_{ee}$ and $\hat{v}_{\mathrm{SCE}}$ are diagonal in the space of Slater Determinants built from the one-particle position eigenstates. That is, we can choose the $|\Psi_P\rangle$ to be $|\boldsymbol{r}_{p_1},\boldsymbol{r}_{p_2},\dots\boldsymbol{r}_{p_N}\rangle = \frac{1}{\sqrt{N!}}|\boldsymbol{r}_{p_1}\rangle\wedge|\boldsymbol{r}_{p_2}\rangle\wedge\dots\wedge|\boldsymbol{r}_{p_N}\rangle$ (including spin where necessary), and where we order the Slater determinants (in any arbitrary way) to prevent overcompleteness.

The resulting ensemble is then given by,

$$\hat{\Gamma} = \int d\boldsymbol{r}_1 d\boldsymbol{r}_2 \dots d\boldsymbol{r}_N w(\boldsymbol{r}_1,\boldsymbol{r}_2,\dots\boldsymbol{r}_N)|\boldsymbol{r}_1,\boldsymbol{r}_2,\dots\boldsymbol{r}_N\rangle\langle\boldsymbol{r}_1,\boldsymbol{r}_2,\dots\boldsymbol{r}_N| \tag{S8}$$

Inserting this result for $\hat{\Gamma}$ back into the Lagrangian and using that the Slater determinants are orthonormal, we recover exactly the Lagrangian of S3, identifying $w(\boldsymbol{r}_1,\boldsymbol{r}_2,\dots\boldsymbol{r}_N)$ with $P_N(\boldsymbol{r}_1,\boldsymbol{r}_2,\dots\boldsymbol{r}_N)$ [1]. This shows that for the strictly correlated limit of ground-state DFT:

$$V_{ee}^{\mathrm{SCE}}[n] = \min_{\Psi\to n}\langle\Psi|\hat{V}_{ee}|\Psi\rangle = \min_{\hat{\Gamma}\to n}\mathrm{Tr}[\hat{\Gamma}\hat{V}_{ee}]. \tag{S9}$$

Note however that the minimizer in both cases is a completely different state, one is a pure state (an ensemble with only a single weight non-zero), while the other in general has many weights not equal to zero.

Since we can obtain the same energy from a pure state or an ensemble with arbitrary weights, it seems likely that a countable number of solutions can be constructed by combining the states from the SCE manifold. That is, all combinations of positions for which,

$$\left(\hat{V}_{ee} + \hat{v}_{\mathrm{SCE}}\right) |\boldsymbol{r}_1 \ldots \boldsymbol{r}_N\rangle = E_{\mathrm{SCE}} |\boldsymbol{r}_1 \ldots \boldsymbol{r}_N\rangle, \tag{S10}$$

where,

$$E_{\mathrm{SCE}} = \min_{\boldsymbol{r}_1 \ldots \boldsymbol{r}_N} \left( \sum_{i<j} \frac{1}{|\boldsymbol{r}_i - \boldsymbol{r}_j|} + v_{\mathrm{SCE}}(\boldsymbol{r}_i) \right) . \tag{S11}$$

The only requirement is that solutions satisfy,

$$\sum_P w_P |\Psi_P(\boldsymbol{r}_1, \boldsymbol{r}_2, \ldots \boldsymbol{r}_N)|^2 = P_N(\boldsymbol{r}_1, \boldsymbol{r}_2, \ldots \boldsymbol{r}_N) . \tag{S12}$$

We will show in the following sections that this condition may be satisfied for any finite or countably infinite number of non-zero weights $w_P$.

### 1. *Constructing the pure state*

We can construct an SCE wavefunction (here we take the fully spin-polarized, but we can generalize to any spin using configuration state functions), with probability density $P_N$ in the following way:

$$\Psi_{\mathrm{SCE}}(\boldsymbol{r}_1, \ldots \boldsymbol{r}_N) = \epsilon(\boldsymbol{r}_1, \ldots \boldsymbol{r}_N) \sqrt{P_N(\boldsymbol{r}_1, \ldots \boldsymbol{r}_N)}, \tag{S13}$$

where $\epsilon$ is function that is anti-symmetric in its arguments such that $|\epsilon(\boldsymbol{r}_1, \ldots \boldsymbol{r}_N)|^2 = 1$ for all arguments, such that $|\Psi_{\mathrm{SCE}}(\boldsymbol{r}_1, \ldots \boldsymbol{r}_N)|^2 = P_N(\boldsymbol{r}_1, \ldots \boldsymbol{r}_N)$. This is not possible if any of the electrons are at the same point, but at these points $P_N$ is sure to be zero, as these are the points where the interaction diverges.

The exact form of $\epsilon$ can only be determined at a higher order, since many choices of $\epsilon$ will satisfy the anti-symmetry conditions. To eliminate the constraint that $|\epsilon(\boldsymbol{r}_1, \ldots \boldsymbol{r}_N)|^2 = 1$ we will parameterize,

$$\epsilon(\boldsymbol{r}_1, \ldots \boldsymbol{r}_N) = e^{i\theta(\boldsymbol{r}_1, \ldots \boldsymbol{r}_N)}, \tag{S14}$$

where now $\theta(\boldsymbol{r}_1, \ldots \boldsymbol{r}_N)$ should now shift by $\pi$ upon an odd permutation of the electrons. Many choices of $\theta$ are possible, only when introducing kinetic energy one is picked.

Intuitively, we expect the phase to be as constant as possible to minimize the kinetic energy, which will contain a contribution from the phase of the form $\sum_{i=1}^{N} |\nabla_{\boldsymbol{r}_i}\theta(\boldsymbol{r}_1, \boldsymbol{r}_2, \dots \boldsymbol{r}_N)|^2$. Indeed, since $P_N$ is always zero when electrons are at the same point, the phase can be constant (either 0 or $\pi$ up to a global phase) on the $N!$ different branches of the degenerate manifold, which correspond to the permutations of the electrons.

*2. Extension and application to ensemble DFT*

In ensemble DFT we have a fixed set of weights, $\boldsymbol{w} = \{w_P\}$, and a density that needs to be constrained. The corresponding SCE functional is defined as,

$$\mathcal{V}_{\text{ee}}^{\text{SCE},\boldsymbol{w}}[n] := V_{ee}^{\text{SCE}}[n, \{w_P\}] := \min_{\hat{\Gamma}\to n} \sum_P w_P \langle \Psi_P | \hat{V}_{ee} | \Psi_P \rangle. \tag{S15}$$

The Lagrangian for the minimization is,

$$\begin{aligned} L_{\text{SCE}}[n, \{w_P\}; v_{\text{SCE}}, \{\epsilon_{PQ}\}] = & \sum_P w_P \langle \Psi_P | \hat{V}_{ee} | \Psi_P \rangle \\ & + \int d\boldsymbol{r} v_{\text{SCE}}(\boldsymbol{r}) \left( \sum_P w_P \langle \Psi_P | \hat{n}(\boldsymbol{r}) | \Psi_P \rangle - n(\boldsymbol{r}) \right) \\ & - \sum_{PQ} \epsilon_{PQ} (\langle \Psi_P | \Psi_Q \rangle - \delta_{PQ}) \,, \end{aligned} \tag{S16}$$

this time using weights $\boldsymbol{w} = \{w_P\}$ as parameters, not variables to be minimized over. From the previous discussion about pure states and ensembles in SCE it is plausible that, regardless of the chosen weights, we will in fact find $V_{\text{ee}}^{\text{SCE}}[n, \{w_P\}] = V_{\text{ee}}^{\text{SCE}}[n]$, and also $v_{\text{SCE}}(\boldsymbol{r})$ will be the same. All that is necessary is that Eq. (S12) is satisfied, which directly implies also the density constraint. The particular partitioning between the different states is only determined at a higher order by the inclusion of the kinetic energy, with the corresponding corrections to the potential to satisfy the density constraint.

One particular option is that,

$$\Psi_P(\boldsymbol{r}_1, \dots \boldsymbol{r}_N) = e^{i\theta_P(\boldsymbol{r}_1, \dots \boldsymbol{r}_N)} \sqrt{P_N(\boldsymbol{r}_1, \dots \boldsymbol{r}_N)}, \tag{S17}$$

where $\theta_P(\boldsymbol{r}_1, \dots \boldsymbol{r}_N)$ is such that the anti-symmetry condition is fulfilled, and,

$$\langle \Psi_P | \Psi_Q \rangle = \int d\boldsymbol{r}_1 \dots d\boldsymbol{r}_N P_N(\boldsymbol{r}_1, \dots \boldsymbol{r}_N) e^{i\left(\theta_Q(\boldsymbol{r}_1, \dots \boldsymbol{r}_N) - \theta_P(\boldsymbol{r}_1, \dots \boldsymbol{r}_N)\right)} = \delta_{PQ} \quad \forall \quad P, Q. \tag{S18}$$

Such a construction is clearly possible for any finite or countably infinite number of non-zero weights, since we can pick $\theta_P$ and $\theta_Q$ to yield positive and negative regions. This choice is enough to prove that the leading term at strong interaction (or low density) is weight independent, but it does not allows us to prove weight-independence at the next leading order. A construction that allows us to do that is presented in the next section.

### B. Weight-independence of the next leading term

We will now switch our attention to the higher order contributions after SCE. The next order is given by the electronic zero-point energy (ZPE), the oscillations around the equilibrium positions given by the degenerate SCE manifold. The correct ZPE treatment is given by a careful expansion of the potential around the minimum, which was developed in [4] and we refer to it for the details.

This treatment will result in identifying the two leading terms of the strong coupling limit of ensemble DFT,

$$\frac{\partial F^\lambda[n,\{w_P\}]}{\partial\lambda} = \tilde{W}_\lambda[n,\{w_P\}] = \tilde{W}_\infty[n,\{w_P\}] + \frac{W'_\infty[n,\{w_P\}]}{\sqrt{\lambda}} + \mathcal{O}(\lambda^{-p}) , \tag{S19}$$

$$F^\lambda[n,\{w_P\}] = \lambda\tilde{W}_\infty[n,\{w_P\}] + \sqrt{\lambda}2W'_\infty[n,\{w_P\}] + O(\lambda^{1-p}), \tag{S20}$$

where we already showed (Section I A 2) that $\tilde{W}_\infty[n,\{w_P\}] = \tilde{W}_\infty[n] := V_{ee}^{\mathrm{SCE}}[n]$ and will proceed to show that $W'_\infty[n,\{w_P\}] = W'_\infty[n] := \frac{1}{2}F^{\mathrm{ZPE}}[n]$. Note, we use $\tilde{W}_\infty$ here to distinguish from the more common notation $W_\infty = \tilde{W}_\infty - E_{\mathrm{H}}[n]$, which is the SCE energy minus the classical Hartree energy, $E_{\mathrm{H}}$. Here, $p \geq \frac{5}{4}$.

The Hamiltonian expanded for large interaction strength $\lambda$ is given by,

$$\hat{H}_\lambda = \lambda E_{\mathrm{SCE}} + \sqrt{\lambda}\hat{H}^{(0)} + \lambda^{1/4}\hat{H}^{(1)} + \hat{H}^{(2)} + \mathcal{O}(\lambda^{-1/4}). \tag{S21}$$

The order $\sqrt{\lambda}$ Hamiltonian, $\hat{H}^{(0)} = \hat{H}_{\mathrm{ZPE}}$ describes the zero-point oscillations. We already know [from eq. (S17)] that at order $\lambda$ we recover the weight-independent $V_{ee}^{\mathrm{SCE}}[n]$. The question is then how the weights enter at higher order, and how we can explicitly construct the ensemble with given weights and density in the limit $\lambda \to \infty$.

From now on we will assume the degenerate SCE manifold $\mathcal{M}$ is of Monge type. That is, given the position of the first electron, we can find the positions of the other electrons by repeated application of a co-motion function $\boldsymbol{f}_i(\boldsymbol{r})$: $\mathcal{M} = \{\boldsymbol{r}, \boldsymbol{f}_2(\boldsymbol{r}), \dots \boldsymbol{f}_N(\boldsymbol{r}) | \forall \boldsymbol{r} \in \mathbb{R}^d\}$,

where $d$ is the dimensionality of space. Given $\boldsymbol{R} = \boldsymbol{r}_1, \boldsymbol{r}_2, \ldots \boldsymbol{r}_N$ we denote the closest point on $\mathcal{M}$ with $\boldsymbol{s}$, and we expand the electrostatic potential on the manifold to second order around,

$$\begin{aligned} E_{\text{pot}}(\boldsymbol{r}_1, \boldsymbol{r}_2, \ldots \boldsymbol{r}_N) =& \sum_{i<j} \frac{1}{|\boldsymbol{r}_i - \boldsymbol{r}_j|} + v_{\text{SCE}}(\boldsymbol{r}_i) \\ =& E_{\text{SCE}} + \frac{1}{2} \sum_{ij} (\boldsymbol{r}_i - \boldsymbol{f}_i(\boldsymbol{s})) \mathsf{H}_{ij}(\boldsymbol{s}) (\boldsymbol{r}_j - \boldsymbol{f}_j(\boldsymbol{s})). \\ =& E_{\text{SCE}} + \frac{1}{2} (\boldsymbol{R} - \boldsymbol{F}(\boldsymbol{s})) \mathbb{H}(\boldsymbol{s}) (\boldsymbol{R} - \boldsymbol{F}(\boldsymbol{s})). \end{aligned} \tag{S22}$$

Here $\mathsf{H}_{ij}$ is a $d \times d$ matrix, which collectively define a Hessian, $\mathbb{H}$. Diagonalizing the Hessian $\mathbb{H}$ yields $d$ zero eigenvalues corresponding to the direction on the manifold; and $d(N-1)$ non-zero eigenvalues corresponding to the directions orthogonal to the manifold.

The eigenmodes define the behaviour of quantum Harmonic oscillators (QHOs). To study their behaviour we switch to a set of curvilinear coordinates, $\boldsymbol{s}$, corresponding to the position on the manifold, and, $\boldsymbol{Q}$, being the deviation from the manifold in terms of the $d(N-1)$ coordinates corresponding to the other eigenvectors of the Hessian at $\boldsymbol{s}$. Scaling in the large $\lambda$ limit, we set $\boldsymbol{U} = \lambda^{1/4} \boldsymbol{Q}$ and find the ZPE Hamiltonian, which is a sum of QHOs in $u_i$:

$$\hat{H}_{\text{ZPE}} = -\frac{1}{2} \sum_{i=4}^{3N} \frac{\partial^2}{\partial u_i^2} + \sum_{i=4}^{3N} \frac{\omega_i(\boldsymbol{s})^2}{2} u_i^2 - \sum_{i=4}^{3N} \frac{\omega_i(\boldsymbol{s})}{2} \; . \tag{S23}$$

For ground-state DFT this is solved via a product of Gaussians $\Phi$ in $u_i$, giving,

$$\Psi_{\text{ZPE}}(\boldsymbol{s}, \boldsymbol{U}) = C^{(0)}(\boldsymbol{s}) \prod_{i=4}^{3N} \Phi_{\omega_i(\boldsymbol{s})}(u_i), \tag{S24}$$

Integrating over $u$ and enforcing the density constraint we find,

$$|C^{(0)}(\boldsymbol{s})|^2 = \frac{1}{N} \frac{n(\boldsymbol{s})}{J(\boldsymbol{s}, \underline{0})}, \tag{S25}$$

where $J(\boldsymbol{s}, \boldsymbol{U})$ is the determinant of the Jacobian corresponding to the transformation to the curvilinear coordinates. The value of $F^{\text{ZPE}}[n]$ can be calculated via the virial theorem for the oscillators to be:

$$F^{\text{ZPE}}[n] = \int d\boldsymbol{s} \frac{n(\boldsymbol{s})}{N} \sum_{i=4}^{3N} \frac{\omega_i(\boldsymbol{s})}{2}. \tag{S26}$$

At this stage, it might be tempting to define excited states by higher excitations of the QHOs, thus obtaining a higher $F^{\text{ZPE}}[n]$ in the ensemble versus the ground-state. Indeed

such a construction leads to $V_{ee}^{\text{SCE}}[n]$ independent of weights, to leading order. However we can realize the ground state of the harmonic oscillator for every state in the ensemble by enforcing orthogonality only through the $\boldsymbol{s}$ coordinate. That is, we take,

$$\Psi_P^{\text{ZPE}}(\boldsymbol{s},\boldsymbol{U}) = \frac{\phi_P(\boldsymbol{s})}{\sqrt{J(\boldsymbol{s},\underline{0})}}\prod_{i=4}^{3N}\Phi_{\omega_i(\boldsymbol{s})}(u_i), \tag{S27}$$

and demand,

$$n(\boldsymbol{s}) = N\sum_P w_P|\phi_P(\boldsymbol{s})|^2 \, , \qquad \int d\boldsymbol{s}\phi_P^*(\boldsymbol{s})\phi_Q(\boldsymbol{s}) = 0 \quad \forall \quad P \neq Q \, . \tag{S28}$$

Provided their energy can be kept finite, which we will show in the following steps, such states will not contribute at $O(\sqrt{\lambda})$ in the energy.

One particular realization of this is the Harriman [5] construction,

$$\phi_P(\boldsymbol{s}) = \sqrt{\frac{n(\boldsymbol{s})}{N}}e^{i\frac{2\pi P}{N}\text{Ne}(\boldsymbol{s})}, \tag{S29}$$

where $P = 0, 1, 2, \ldots$ and $\text{Ne}(\boldsymbol{s}) = \int_{-\infty}^{s} \mathrm{d}x' n(x')$ is the cumulant of the density $n(\boldsymbol{s})$. We illustrate the construction for $d = 1$, but it can be easily extended to $d = 3$ as discussed by Harriman. This construction automatically maintains orthonormality because,

$$\frac{1}{N}\int_{-\infty}^{\infty} ds n(s) e^{i\frac{2\pi(Q-P)}{N}\text{Ne}(s)} = \frac{1}{N}\int_0^N e^{i\frac{2\pi(Q-P)}{N}\text{Ne}} d\text{Ne} = \delta_{PQ}. \tag{S30}$$

Because we can do this construction for any finite or countably infinite number of weights, we conclude that $\mathcal{V}_{ee}^{\text{SCE},\boldsymbol{w}}[n] = V_{ee}^{\text{SCE}}[n,\{w_P\}] = V_{ee}^{\text{SCE}}[n]$ and $\mathcal{F}^{\text{ZPE},\boldsymbol{w}}[n] = F^{\text{ZPE}}[n,\{w_P\}] = F^{\text{ZPE}}[n]$, as long as the contribution at the next order remains finite. To show that its energy contribution is finite, we need to determine $\{\phi_P\}$ and then evaluate energies of states defined by eq. (S27), which we shall proceed to do.

To obtain $\{\phi_P(\boldsymbol{r})\}$ we need to look at the higher order contributions in the Hamiltonian, $\hat{H}^{(1)}$ and $\hat{H}^{(2)}$, and minimize their expectation value. The non-constant terms in $\hat{H}^{(1)}$ are odd in $u_i$ or $\frac{\partial}{\partial u_i}$ and therefore yield zero as an expectation value on all of the $|\Psi_P^{\text{ZPE}}\rangle$. The constant terms only depend on normalization, and so are the same for all $|\Psi_P^{\text{ZPE}}\rangle$.

Therefore, to show that the ensemble energy at the next order remains finite, we can restrict our attention to $\hat{H}^{(2)}$. The potential energy depends only on,

$$\sum_P w_P|\Psi_P^{\text{ZPE}}(\boldsymbol{s},\boldsymbol{U})|^2 = \frac{1}{J(\boldsymbol{s},\underline{0})}|\prod_{i=4}^{3N}\Phi_{\omega_i(\boldsymbol{s})}(u_i)|^2\sum_P w_P|\phi_P(\boldsymbol{s})|^2 = \frac{n(\boldsymbol{s})}{NJ(\boldsymbol{s},\underline{0})}|\prod_{i=4}^{3N}\Phi_{\omega_i(\boldsymbol{s})}(u_i)|^2, \tag{S31}$$

and therefore is independent of $\{\phi_P(\boldsymbol{s})\}$, as expected. We are only left with the kinetic energy contributions $\hat{T}^{(2)}$, which has a rather formidable expression given in Appendix A of Ref [6]. However, many terms in $\hat{T}^{(2)}$ yield an expectation value that is either zero, or independent of the choice of $\{\phi_P(\boldsymbol{s})\}$, in particular any terms that do not contain any derivatives towards $\boldsymbol{s}$. The Lagrangian we need to solve for $\{\phi_P(\boldsymbol{s})\}$ is then,

$$\begin{aligned} L^{(2)}[n, \{w_P\}; v^{(2)}, \{\phi_P\}, \{\epsilon^{(2)}_{PQ}\}] = &\sum_P w_P \langle \Psi_P^{\text{ZPE}} | \Delta\hat{T}^{(2)} | \Psi_P^{\text{ZPE}} \rangle \\ &+ \int d\boldsymbol{s} v^{(2)}(\boldsymbol{s}) \left( \sum_P w_P |\phi_P(\boldsymbol{s})|^2 - \frac{n(\boldsymbol{s})}{N} \right) \\ &- \sum_{PQ} \epsilon^{(2)}_{PQ} \left( \int d\boldsymbol{s} \phi_P^*(\boldsymbol{s}) \phi_Q(\boldsymbol{s}) - \delta_{PQ} \right), \end{aligned} \tag{S32}$$

where $\Delta\hat{T}^{(2)}$ consists only of the following terms,

$$\Delta\hat{T}^{(2)} = -\frac{1}{2} \sum_{\alpha,\beta=1,2,3} g^{\alpha\beta} \frac{\partial}{\partial s_\alpha \partial s_\beta} - \frac{1}{2} \sum_{\alpha,\beta=1,2,3} \left( \frac{g^{\alpha\beta}}{2\det(g)} \frac{\partial \det(g)}{\partial s_\beta} + \frac{\partial g^{\alpha\beta}}{\partial s_\beta} \right) \frac{\partial}{\partial s_\alpha}, \tag{S33}$$

where $g^{\alpha\beta}$ is the inverse metric, $\det g$ is the determinant of the metric, and both depend on the coordinate $\boldsymbol{s}$. Explicitly the metric is given by,

$$g_{\alpha\beta}(\boldsymbol{s}) = \sum_{i=1}^{N} \frac{\partial \boldsymbol{f}_i(\boldsymbol{s})}{\partial s_\alpha} \cdot \frac{\partial \boldsymbol{f}_i(\boldsymbol{s})}{\partial s_\beta}. \tag{S34}$$

By making use of partial differentiation we can obtain a simpler expression for the symmetrized operator,

$$\Delta\hat{T}^{(2)} = \frac{1}{2} \overleftarrow{\frac{\partial}{\partial s^\beta}} g^{\alpha\beta} \overrightarrow{\frac{\partial}{\partial s^\alpha}}, \tag{S35}$$

in the space weighted by $J(\boldsymbol{s}, \underline{0}) = \sqrt{\det g}|_{\boldsymbol{U}=\underline{0}}$.

We finally need to compute the integral,

$$\langle \Psi_P | \Delta\hat{T}^{(2)} | \Psi_P \rangle = \frac{1}{2} \int d\boldsymbol{s} J(\boldsymbol{s}, \underline{0}) \sum_{\alpha,\beta} \frac{\partial \frac{\phi_P(\boldsymbol{s})^*}{\sqrt{J(\boldsymbol{s})}}}{\partial s_\beta} g^{\alpha\beta} \frac{\partial \frac{\phi_P(\boldsymbol{s})}{\sqrt{J(\boldsymbol{s})}}}{\partial s_\alpha}, \tag{S36}$$

to obtain,

$$\Delta\mathcal{T}^{(2),\boldsymbol{w}}[n] := \sum_P w_P \langle \Psi_P | \Delta\hat{T}^{(2)} | \Psi_P \rangle \tag{S37}$$

With this we have every ingredient of the Lagrangian of equation S32. Doing the variation w.r.t. $\phi_P^*(\boldsymbol{s})$ yields an effective "single-particle" Schrödinger equation corresponding to the

collective movement of the electrons. It only differs from the usual single-particle Schrödinger equation in that the kinetic energy operator takes a somewhat complicated form. Despite this, it is expected that, just like in the usual case, for any arbitrary number of weights we can find a solution to the Lagrangian with a finite expectation value of the kinetic energy. That is, we assume the single-particle equation to have infinitely many solutions with a finite energy.

The fact that the we can construct an ensemble where the weight dependence enters only at the order $\lambda^0$ of the energy and always yields a finite contribution shows that indeed the contribution at order $\lambda$ ($V_{\rm ee}^{\rm SCE}[n]$) and order $\sqrt{\lambda}$ ($F^{\rm ZPE}[n]$) are weight independent. To summarize, the effect of weights only enters at $O(\lambda^0) = O(1)$, yielding,

$$\mathcal{F}^{\lambda,\boldsymbol{w}}[n] = \mathcal{F}^{\lambda}[n, \{w_P\}] = \lambda V_{ee}^{\rm SCE}[n] + \sqrt{\lambda} F^{\rm ZPE}[n] + O(1) , \tag{S38}$$

where the weight-dependent $O(1)$ term is related to eq. (S37).

## II. HARMONIUM ATOMS

The manuscript reports exact results on Harmonium atoms. In this section, we detail the Hamlitonians, theory and numerical methods used to produce key results.

### A. Proof that interaction energies become classical

We will show that the solutions, $|\Psi_\kappa^\lambda\rangle$ of $\hat{H}|\Psi_\kappa^\lambda\rangle = E_\kappa^\lambda|\Psi_\kappa^\lambda\rangle$ of the Hamiltonian,

$$\hat{H} = \left\{ \sum_{j=1}^{N} \frac{1}{2}[-\nabla_j^2 + \boldsymbol{r}_j^2] + \sum_{i=1,j<i}^{N} \frac{\lambda}{|\boldsymbol{r}_i - \boldsymbol{r}_j|} \right\} := \{\hat{T} + \hat{v}_{\rm ext} + \lambda \hat{V}_{ee}\} , \tag{S39}$$

obey $\lim_{\lambda\to\infty}\langle\Phi_\kappa^\lambda|\hat{V}_{ee}|\Phi_\kappa^\lambda\rangle = V_{\rm cl}^\lambda$, where $V_{\rm cl}^\lambda$ is the classical energy defined below.

We begin with the classical solution, which is the minimum of $E(\{\boldsymbol{r}\}) = \frac{1}{2}\sum_i \boldsymbol{r}_i^2 + \sum_{j<j} \frac{\lambda}{|\boldsymbol{r}_i - \boldsymbol{r}_j|}$ for point charges located at $\boldsymbol{r}_i$ (i.e. $\hat{H}$ without the Laplacian). The solution may be found by minimizing, $E^\lambda(R) = \frac{1}{2}NR^2 + \frac{\lambda N\bar{w}(N)}{R}$, giving,

$$R_{\rm cl}^\lambda = \bar{w}(N)^{1/3}\lambda^{1/3} , \quad E_{\rm cl}^\lambda = E^\lambda(R_{\rm cl}^\lambda) = \tfrac{3}{2}N\bar{w}(N)^{2/3}\lambda^{2/3} , \quad V_{\rm cl}^\lambda = \tfrac{N\bar{w}(N)}{R_{\rm cl}^\lambda} = \tfrac{N\bar{w}(N)^{2/3}}{\lambda^{1/3}} \tag{S40}$$

as the important minimizing values. Here,

$$N\bar{w}(N) = \min_{\boldsymbol{X},\|\boldsymbol{X}\|=N} V_{ee}(\boldsymbol{X}) , \qquad V_{ee}(\boldsymbol{X}) = \sum_{i=1,j<i}^{N} \frac{1}{|\boldsymbol{x}_i - \boldsymbol{x}_j|} , \tag{S41}$$

is the minimum electrostatic energy of $N$ point charges located at vectors of average unit length, i.e. that $\|\boldsymbol{X}\| = N$ where $\boldsymbol{X} = \{\boldsymbol{x}\}_{i=1}^{N}$. Note, the classical formulae used in the main text are examples of this approach.

We next select some $\boldsymbol{X}_0(N) \in \arg\min V_{ee}(\boldsymbol{X})$ to obtain the Taylor expansion,

$$\tilde{E}^{\lambda}(\boldsymbol{R}) \approx E^{\lambda}_{\text{cl}} + \tfrac{1}{2}K_{RR}(R - R^{\lambda}_{\text{cl}})^2 + \tfrac{1}{2}(\boldsymbol{R} - \boldsymbol{R}_0) \cdot \mathsf{K}_{\perp} \cdot (\boldsymbol{R} - \boldsymbol{R}_0) \,, \tag{S42}$$

where $K_{RR} = 3N$, $\boldsymbol{R}_0 = R^{\lambda}_{\text{cl}}\boldsymbol{X}_0(N)$ and $\mathsf{K}_{\perp} := \Omega^2_{\perp} \propto \lambda/R^{\lambda}_{\text{cl}} \propto N^{1/3}\lambda^{2/3}$ involves second derivatives of $N\bar{w}(N)$ around $\boldsymbol{X}_0(N)$. Note, $\mathsf{K}_{\perp}$ and $\Omega^2_{\perp}$ have three zero eigenvalues, one for $R$ and two because rotations around the unit sphere do not change the electrostatic energy.

Reintroducing the kinetic energy to obtain, $\hat{H}^{\lambda} \approx \sum_{i=1}^{N} -\frac{1}{2}\nabla^2_i + \tilde{E}^{\lambda}(\{\boldsymbol{R}\})$ then yields,

$$E^{\lambda}_{\kappa} \approx E^{\lambda}_{\text{cl}}\big[1 + A_{\perp}(N)\big] + \frac{2\kappa + 1}{2}\sqrt{3N} \tag{S43}$$

for the $\kappa$th lowest energy QHO as $\lambda \to \infty$, where $A_{\perp}(N) = \frac{1}{2}\text{Tr}[\Omega_{\perp}]/E^{\lambda}_{\text{cl}}$ collects the zero point energies for high energy oscillations around the hypersphere and the last term is for lower energy radial fluctuations around $R^{\lambda}_{\text{cl}}$. The wave function is,

$$\Psi^{\lambda}_{\kappa}(\boldsymbol{R}) \propto q_{\kappa}(\sqrt{3N}(R - R^{\lambda}_{\text{cl}}))\hat{\mathcal{A}}e^{-(\boldsymbol{R}-\boldsymbol{R}_0)\cdot\Omega_{\perp}\cdot(\boldsymbol{R}-\boldsymbol{R}_0)} \,, \tag{S44}$$

where $\hat{\mathcal{A}}$ introduce the appropriate Fermionic anti-symmetry. Here, $q_{\kappa}$ is the $\kappa$th solution of a QHO with $\omega = \sqrt{3N}$. We remind that $\Omega_{\perp}$ has three zero eigenvalues.

Importantly, as $\lambda \to \infty$ all the oscillators except $q_{\kappa}$ become very localised because $\Omega_{\perp} \propto \lambda^{1/3}$. This means they may be approximated by Dirac $\delta$ functions centered at their classical values, and that Fermionic effects can be ignored in the wavefunction. Thus,

$$\lim_{\lambda\to\infty} \langle \Phi^{\lambda}_{\kappa}|\hat{V}_{ee}|\Phi^{\lambda}_{\kappa}\rangle = \bar{w}(N)\int \frac{q_{\kappa}(\sqrt{3N}(R - R^{\lambda}_{\text{cl}}))}{R}d\boldsymbol{R} \tag{S45}$$

$$\approx \frac{\bar{w}(N)}{R^{\lambda}_{\text{cl}}}\int q_{\kappa}(\sqrt{3N}(R - R^{\lambda}_{\text{cl}}))\left[1 + \frac{R^{\lambda}_{\text{cl}} - R}{R^{\lambda}_{\text{cl}}} + \frac{(R^{\lambda}_{\text{cl}} - R)^2}{(R^{\lambda}_{\text{cl}})^2}\right]d\boldsymbol{R} \tag{S46}$$

$$= V^{\lambda}_{\text{cl}}\big[1 + \tfrac{b_{\kappa}}{N(R^{\lambda}_{\text{cl}})^2}\big] \,. \tag{S47}$$

where we used that $q_{\kappa}$ is centered at $R^{\lambda}_{\text{cl}} \propto \lambda^{1/3}$ with much smaller width $\propto N^{-\frac{1}{2}} \ll R^{\lambda}_{\text{cl}}$. The first term is the classical solution and the second decays faster as $V^{\lambda}_{\text{cl}}\lambda^{-2/3} \propto \lambda^{-1}$. Thus, we see that, $\lim_{\lambda\to\infty}\langle \Phi^{\lambda}_{\kappa}|\hat{V}_{ee}|\Phi^{\lambda}_{\kappa}\rangle = V^{\lambda}_{\text{cl}}$.

## B. Two electrons in 3D

The 3D Harmonium atom with two electrons obeys the Hamiltonian,

$$\hat{H}(\lambda)\Psi_\kappa^\lambda(\boldsymbol{r}_1,\boldsymbol{r}_2) = E_\kappa^\lambda\Psi_\kappa^\lambda(\boldsymbol{r}_1,\boldsymbol{r}_2) \; , \tag{S48}$$

$$\hat{H}(\lambda) := \frac{1}{2}\big[-\nabla_1^2 + \boldsymbol{r}_1^2\big] + \frac{1}{2}\big[-\nabla_2^2 + \boldsymbol{r}_2^2\big] + \frac{\lambda}{|\boldsymbol{r}_1 - \boldsymbol{r}_2|} \; . \tag{S49}$$

We report only spherically symmetric eigen-solutions of S48. These are found by changing variables to $\boldsymbol{X} = \frac{1}{\sqrt{2}}[\boldsymbol{r}_1 + \boldsymbol{r}_2]$ and $\boldsymbol{R} = \frac{1}{\sqrt{2}}[\boldsymbol{r}_1 - \boldsymbol{r}_2]$ so that $\Psi_\kappa^\lambda(\boldsymbol{X},\boldsymbol{R}) := q_{s_\kappa}(X)\psi_{t_\kappa}^\lambda(R)$ (because of symmetry) and $E_\kappa := e_{s_\kappa}^q + e_{t_\kappa}^{\psi,\lambda}$. The separated solutions obey,

$$\left[\frac{-1}{2X}\frac{\partial^2}{\partial X^2}X + \frac{1}{2}X^2\right]q_s(X) := e_s^q q_s(X) \; , \tag{S50}$$

$$\left[\frac{-1}{2R}\frac{\partial^2}{\partial R^2}R + \frac{1}{2}R^2 + \frac{\lambda}{\sqrt{2}R}\right]\psi_t^\lambda(R) := e_t^{\psi,\lambda}\psi_t^\lambda(R) \; . \tag{S51}$$

We work with real-valued solutions. States obeying $\psi_t(R) := \psi_t(-R)$ are triplets, while those obeying $\psi_t(R) = -\psi_t(-R)$ are singlets.

Clearly, $q_s(X)$ are solutions of the spherical quantum harmonic oscillator, with energies $e_s = \frac{1}{2} + S(s)$ where $S(s)$ indicates integers allowed by the symmetry. The solutions $\psi_t^\lambda$ and their eigenvalues $e_t^{\psi,\lambda}$ may be found numerically. Then, the energies $E_\kappa^\lambda = e_{s_\kappa}^q + e_{t_\kappa}^{\psi,\lambda}$ are used to order $s,t$ pairs within the triplet/singlet symmetry groups. Interaction energies are, $V_\kappa^\lambda := \int \psi_{t_\kappa}^\lambda(R)^2\frac{1}{\sqrt{2}R}4\pi R^2 dR$. Densities are found using,

$$n_\kappa^\lambda(\boldsymbol{r}) = 2\int |\Psi_\kappa^\lambda(\tfrac{\boldsymbol{r}+\boldsymbol{r}'}{\sqrt{2}},\tfrac{\boldsymbol{r}-\boldsymbol{r}'}{\sqrt{2}})|^2 d\boldsymbol{r}' = 2\int q_{s_\kappa}(\tfrac{|\boldsymbol{r}+\boldsymbol{r}'|}{\sqrt{2}})^2\psi_{t_\kappa}^\lambda(\tfrac{|\boldsymbol{r}-\boldsymbol{r}'|}{\sqrt{2}})^2 d\boldsymbol{r}' \; . \tag{S52}$$

All numerical calculations are carried out on an even grid using five-point finite difference to evaluate second derivatives – we use symmetric or anti-symmetric boundary conditions to determine values when $r < 0$. We use 128 abscissae, $r_k = h(k + \frac{1}{2})$ for $k \in (0 \ldots 127)$ and $h = 0.1$, to span $r \in [0, 12.8]$. Integrals are evaluated using $I[f] \approx h\sum_{j=0}^{127} f(r_j)$. Numerical errors are expected to be $O(h^2)$ from quadrature.

# III. SCALING TO LOW DENSITIES

This section details the scaling approach used to convert the kinetic energy behaviour at large $\lambda$ to a low-density series expansion.

To begin, we note that eqs. (3) and (9) of the main text give scaling laws,

$$\mathcal{F}^{\lambda,\boldsymbol{w}}[n_\gamma] = \gamma^2 \mathcal{F}^{\lambda/\gamma,\boldsymbol{w}}[n] \qquad \mathcal{F}^{\lambda,\boldsymbol{w}}[n] = \gamma^{-2} \mathcal{F}^{\lambda\gamma,\boldsymbol{w}}[n_\gamma]$$

$$V_{ee}^{\mathrm{SCE}}[n_\gamma] = \gamma V_{ee}^{\mathrm{SCE}}[n] \qquad V_{ee}^{\mathrm{SCE}}[n] = \gamma^{-1} V_{ee}^{\mathrm{SCE}}[n_\gamma] \; .$$

It is then (e.g.) straightforward to derive eq. (8) from the ACF [eq. (5)] using,

$$\begin{aligned} \mathcal{F}^{1,\boldsymbol{w}}[n_\gamma] &= \gamma^2 \mathcal{T}_s[n] + \gamma^2 \int_0^{1/\gamma} \mathcal{V}_{ee}^{\lambda,\boldsymbol{w}}[n] d\lambda \\ &\underset{\gamma\to 0^+}{\longrightarrow} \gamma^2 \int_0^{1/\gamma} \mathcal{V}_{ee}^{\lambda',\boldsymbol{w}}[n] d\lambda' = \gamma \mathcal{V}_{ee}^{\infty,\boldsymbol{w}}[n] = \gamma V_{ee}^{\mathrm{SCE}}[n] = V_{ee}^{\mathrm{SCE}}[n_\gamma] \; . \end{aligned} \tag{S53}$$

In the second line we replaced the integral by $\frac{1}{\gamma} V_{ee}^{\mathrm{SCE}}[n]$ by using $\mathcal{V}_{ee}^{\lambda}[n] \geq \mathcal{V}_{ee}^{\infty}[n]$ and $\lim_{\lambda\to\infty} \mathcal{V}_{ee}^{\lambda}[n] \to V_{ee}^{\mathrm{SCE}}[n]$.

Ensemblizing known results [4, 7, 8] gives $F^{\mathrm{ZPE}} = \mathcal{F}^{\mathrm{ZPE},\boldsymbol{w}} = \lim_{\lambda\to\infty} \frac{\mathcal{F}^{\lambda,\boldsymbol{w}} - \lambda V_{ee}^{\mathrm{SCE}}}{\sqrt{\lambda}}$ which leads immediately to,

$$\begin{aligned} F^{\mathrm{ZPE}}[n_\gamma] &= \lim_{\lambda\to\infty} \frac{\mathcal{F}^{\lambda,\boldsymbol{w}}[n_\gamma] - \lambda V_{ee}^{\mathrm{SCE}}[n_\gamma]}{\sqrt{\lambda}} = \lim_{\lambda\to\infty} \frac{\gamma^2 \mathcal{F}^{\lambda/\gamma,\boldsymbol{w}}[n] - \lambda\gamma V_{ee}^{\mathrm{SCE}}[n]}{\sqrt{\lambda}} \\ &= \gamma^2 \lim_{\lambda\to\infty} \frac{\mathcal{F}^{\lambda/\gamma,\boldsymbol{w}}[n] - \lambda/\gamma V_{ee}^{\mathrm{SCE}}[n]}{\sqrt{\lambda/\gamma}\sqrt{\gamma}} = \gamma^{3/2} \lim_{\lambda\to\infty} \frac{\mathcal{F}^{\lambda,\boldsymbol{w}}[n] - \lambda V_{ee}^{\mathrm{SCE}}[n]}{\sqrt{\lambda}} \\ &= \gamma^{3/2} F^{\mathrm{ZPE}}[n] \; . \end{aligned} \tag{S54}$$

To understand the scaling limit of $\mathcal{T}^{\mathrm{SCE},\boldsymbol{w}}$ we first use the known scaling law, $\mathcal{T}^{\lambda,\boldsymbol{w}}[n_\gamma] = \gamma^2 \mathcal{T}^{\lambda/\gamma,\boldsymbol{w}}[n]$, to obtain the scaling relationship,

$$\mathcal{T}^{\mathrm{SCE},\boldsymbol{w}}[n_\gamma] = \int_1^\infty \frac{\mathcal{T}^{\lambda}[n_\gamma]}{\lambda^2} d\lambda = \int_1^\infty \frac{\mathcal{T}^{\lambda/\gamma,\boldsymbol{w}}[n]}{(\lambda/\gamma)^2} d\lambda = \gamma \int_{1/\gamma}^\infty \frac{\mathcal{T}^{\bar\lambda,\boldsymbol{w}}[n]}{\bar\lambda^2} d\bar\lambda \; .$$

Then, we use the high-density expansion, $\mathcal{T}^{\lambda\to\infty,\boldsymbol{w}} = \frac{\sqrt{\lambda}}{2} F^{\mathrm{ZPE}}$, to show

$$\lim_{\gamma\to\infty} \mathcal{T}^{\mathrm{SCE},\boldsymbol{w}}[n_\gamma] = \gamma \int_{1/\gamma}^\infty \frac{\sqrt{\lambda} F^{\mathrm{ZPE}}[n]}{2\lambda^2} d\lambda = \gamma^{3/2} F^{\mathrm{ZPE}}[n] = F^{\mathrm{ZPE}}[n_\gamma] \; , \tag{S55}$$

which is independent of the ensemble weights, $\boldsymbol{w}$, and appears at $O(\gamma^{3/2})$ in energy.

Our final task is to show that the weight-dependent kinetic energy term decays as $\gamma^2$ for small $\gamma$. This may be seen by defining, $\mathcal{T}^{\lambda,\boldsymbol{w}}[n] := \frac{\sqrt{\lambda}}{2} F^{\mathrm{ZPE}}[n] + \Delta\mathcal{T}^{\lambda,\boldsymbol{w}}[n]$ where $\Delta\mathcal{T}^{\lambda,\boldsymbol{w}}[n] = O(1)$ follows from the Harriman construction. Then,

$$\begin{aligned} \frac{\mathcal{T}^{\lambda,\boldsymbol{w}}[n_\gamma]}{\gamma^2} &= \mathcal{T}^{\lambda/\gamma,\boldsymbol{w}}[n] = \frac{\sqrt{\lambda/\gamma}}{2} F^{\mathrm{ZPE}}[n] + \Delta\mathcal{T}^{\lambda/\gamma,\boldsymbol{w}}[n] \\ \mathcal{T}^{\mathrm{SCE},\boldsymbol{w}}[n_\gamma] &= \gamma^{3/2} F^{\mathrm{ZPE}}[n] + \gamma^2 \int_1^\infty \frac{\Delta\mathcal{T}^{\lambda/\gamma,\boldsymbol{w}}[n]}{\lambda^2} d\lambda \end{aligned}$$

where we recognise that the final integral is $O(1)$, meaning the leading order weight-dependent term is $O(\gamma^2)$. We thus obtain eq. (11) of the main text.

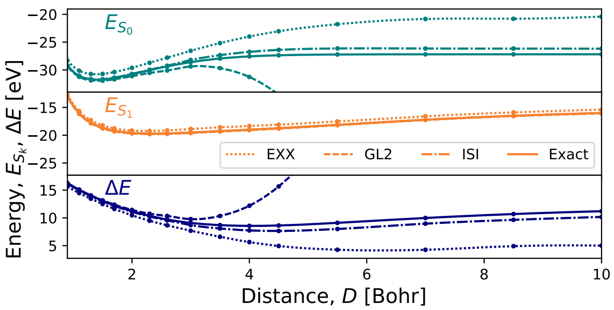


SUPPLEMENTARY FIGURE 1: Ensemblized EXX (dots), GL2 (dashes), ISI (dash-dot) and exact (lines) energies for dissociating $H_2$. Shows ground state energies, $E_{S_0}$, (top, teal), first excited state energies, $E_{S_1}$, (middle, orange) and excitation energies, $\Delta E = E_{S_1} - E_{S_0}$ (bottom, navy). Dots indicate computed values. Extended version of Figure 2 of the main text.

## IV. TECHNICAL DETAILS FOR THE EXCITED STATE CALCULATIONS

### A. $H_2$ dissociation

We use full configuration interaction (FCI) values for 'exact' reference energies, $E_{S_0}$ and $E_{S_1}$, of the lowest two states of dissociating $H_2$, computed using psi4. [9] These calculations also yield accurate FCI reference densities, $n_{S_0}$ and $n_{S_1}$, for states $|S_0\rangle$ and $|S_1\rangle$. All calculations employ a def2-tzvp basis set, [10] that is more than sufficient for our purposes.

To obtain the exact exchange (EXX), Görling-Levy [11] second order energy (GL2), and interaction strength interpolation (ISI) results, we first invert the FCI densities. This yields exact KS orbitals for the gerade ($\phi_h^{S_k}$) and ungerade ($\phi_l^{S_k}$) states; and also the exact Hxc potential, $v_{\rm Hxc}^{S_k}$ which we use to approximate $v_{\rm Hx}^{S_k}$. Note, $2|\phi_h^{S_0}|^2 = n_{S_0}$ and $|\phi_h^{S_1}|^2 + |\phi_l^{S_1}|^2 = n_{S_1}$ (note, $\phi_h^{S_0} \neq \phi_h^{S_1}$). These results then let us compute, $T_{s,S_0} + E_{{\rm Ext},S_0} = 2H_{0,h}^{S_0}$ and $T_{s,S_1} + E_{{\rm Ext},S_1} = H_{0,h}^{S_1} + H_{0,l}^{S_1}$, where $H_{0,k}^{S_k} = \langle \phi_k^{S_k} | \hat{t} + v | \phi_k^{S_k} \rangle$.

Next, we take advantage of the fact that we can use EDFT to directly access properties of $S_0$ and $S_1$, by defining $E_{S_k} := \partial_{w_k} \mathcal{E}^w$. Exact H and x energies for $|S_{0,s}\rangle := |h^\uparrow h^\downarrow\rangle$ and $|S_{1,s}\rangle := \frac{1}{2^{1/2}}[|h^\uparrow l^\downarrow\rangle - |h^\downarrow l^\uparrow\rangle]$ are obtained from the fluctuation-dissipation theorem (FDT): [12]

$$E_{{\rm H},S_{0,s}}^{\rm FDT} = 2(hh|hh) \,, \qquad E_{{\rm H},S_{1,s}}^{\rm FDT} = \tfrac{1}{2}[(hh|hh) + 2(hh|ll) + (ll|ll) + 4(hl|lh)] \,, \tag{S56}$$

$$E_{{\rm x},S_0}^{\rm FDT} = -(hh|hh) \,, \qquad E_{{\rm x},S_1}^{\rm FDT} = -\tfrac{1}{2}[(hh|hh) + 2(hl|lh) + (ll|ll)] \,. \tag{S57}$$

Here, $(ab|cd) = \int \frac{d\boldsymbol{r} d\boldsymbol{r}'}{|\boldsymbol{r}-\boldsymbol{r}'|} \phi_a(\boldsymbol{r})\phi_b(\boldsymbol{r})\phi_c(\boldsymbol{r}')\phi_d(\boldsymbol{r}')$ (all our orbitals are real-valued). Here, and

henceforth, we have stopped the pedantic mention of $S_k$ in the superscript – the orbital choice is instead specified by the context. Then, applying Görling-Levy (GL2) second order perturbation theory to the ensemble states yields,

$$E^{\rm GL2}_{{\rm c},S_0} \approx \sum_{cd\neq hh} \frac{|(hc|hd) - \bar{v}_{hc,hd} - \bar{v}_{hd,hc}|^2}{R(2\epsilon_h - \epsilon_c - \epsilon_d)} , \quad E^{\rm GL2}_{{\rm c},S_1} \approx \frac{1}{2} \sum_{cd\neq hl,lh} \frac{|(hc|ld) + (lc|hd) - \bar{V}_{hl,cd}|^2}{R(\epsilon_h + \epsilon_l - \epsilon_c - \epsilon_d)} , \tag{S58}$$

for the correlation energies. Here, $\bar{v}_{ab,cd} = \langle\phi_a|v^w_{\rm Hxc}|\phi_b\rangle\delta_{cd}$ and $\bar{V}_{ab,cd} = \bar{v}_{ac,bd} + \bar{v}_{bd,ac} + \bar{v}_{bd,ad} + \bar{v}_{ad,bc}$. $R(E)$ is a numerical correction that will be discussed below.

GL2 perturbation theory is well-defined in ground states and excited-state enesembles, [11, 13] and can be rigorously exteneded to symmetry-induced degeneracies so long as one ensures that all degenerate states are equally weighted. [14, 15] However, the GL2 correlation energies reveal a *practical* problem with using inverted properties in the denominator that warrants some additional discussion: although the orbitals are robust against numerical noise, their energies, $\epsilon_k$, are not due to basis set over/undercompleteness issues. This is especially problematic when $\epsilon_l - \epsilon_h$ is small, as in the nearly-degenerate gerade and ungerade orbitals of dissociating $H_2$, because transitions from $h$ to $l$ become dominant in the GL2 correlation energy, with a prefactor $\propto \frac{1}{\epsilon_l - \epsilon_h}$. To overcome numerical errors we instead use orbital energies, $\epsilon_k$, from self-consistent PBE ground states, rather than inversion. We also set $R(E) = E/[1 - e^{-(E/0.1\ {\rm mHa})^2}]$ rather than the correct $R(E) = E$ to eliminate any additional issues from the nearly-degenerate states. This numerical trick is similar to regularization approaches already used to improve approximations based on Möller-Plesset perturbation theory. [16]

We are now ready to compute energies. The EXX and GL2 total energies are,

$$E^{\rm EXX}_{S_k} = T_{s,S_k} + E_{{\rm Ext},S_k} + E^{\rm FDT}_{{\rm H},S_k} + E^{\rm FDT}_{{\rm x},S_k} , \qquad E^{\rm GL2}_{S_k} = E^{\rm EXX}_{S_k} + E^{\rm GL2}_{{\rm c},S_k} , \tag{S59}$$

which, because they involve expansion in small $\lambda \sim \gamma^{-1}$, are consistent with series expansions around the high-density limit. The ISI energies are,

$$E^{\rm ISI}_{S_k} = T_{s,S_k} + E_{{\rm Ext},S_k} + E^{\rm FDT}_{{\rm H},S_k} + E^{\rm ISI}_{\rm xc}(E_{{\rm Hx},S_k}, 2E^{\rm GL2}_{{\rm c},S_k}, W_{\infty,S_k}, W'_{\infty,S_k}) . \tag{S60}$$

where the ISI xc approximation, $E^{\rm ISI}_{\rm xc}(W_0, W'_0, W_\infty, W'_\infty)$, is given in eqs (27) and (28) of Ref. [17] [repeated in eq. (S61) and discussed below]. The ISI incorporates the high-density limit via, $E^{\rm FDT}_{{\rm H},S_k}$, $E^{\rm FDT}_{{\rm x},S_k}$ and $E^{\rm GL2}_{{\rm c},S_k}$, which are the same as in GL2. The low-density limit

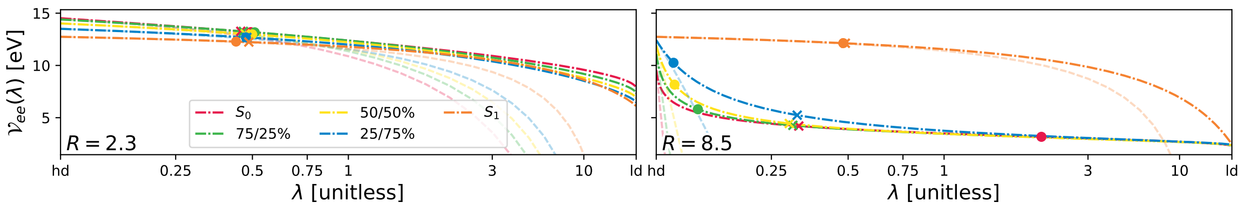


SUPPLEMENTARY FIGURE 2: ISI model interaction strength curves (dash-dot) for different mixtures of ground and excited states ($S_0/S_1$) of $H_2$. Crosses indicate the integrated value, i.e. $\mathcal{E}_{\rm Hxc}^{{\rm ISI},w}$. Dots show the exact $\mathcal{E}_{\rm Hxc}$, for comparison. The faint lines (dashed) show equivalent GL2 curves. Left plot is for a weakly correlated (high-density-like) bonded molecule, while right plot is for strongly correlated (low-density-like) dissociated $H_2$.

is included via harmonium point charge plus continuum (hPC and hPC') gradient density functional approximations, [18] giving $W_{\infty,S_k} = E_{\rm H}[n_{S_k}] + W^{\rm hPC}[n_{S_k}]$ [for classical Hartree energy, $E_{\rm H}[n] = \int \frac{d\boldsymbol{r}d\boldsymbol{r}'}{2|\boldsymbol{r}-\boldsymbol{r}'|} n(\boldsymbol{r})n(\boldsymbol{r}')$] and $W'_{\infty,S_k} = W'^{\rm hPC}[n_{S_k}]$ in terms of FCI densities.

### 1. *Details of the interaction strength interpolation*

To further explore the importance of using both limits in fits, Supplementary Figure 2 shows the model interaction curves of ISI for different ensembles, $\hat{\Gamma} = (1-w)|S_0\rangle\langle S_0| + w|S_1\rangle\langle S_1|$, of $H_2$. Specifically, the plots show,

$$\mathcal{V}_{ee}^{\lambda,w} \approx E_{\rm H}[n^w] + W^{\rm hPC}[n^w] + \frac{2X}{Y}\Big[\sqrt{1+Y} - 1 - Z\log\frac{Z+1}{Z+\sqrt{1+Y}}\Big] \tag{S61}$$

using $X = xy^2/z^2$, $Y = x^2y^2/z^4$ and $Z = xy^2/z^3 - 1$ where $x = -4\mathcal{E}_{\rm c}^{{\rm GL2},w}[n^w]$, $y = W'^{\rm hPC}[n^w]$ and $z = \mathcal{E}_{\rm Hx}^w[n^w] - E_{\rm H}[n^w] - W^{\rm hPC}[n^w]$. Here $n^w = (1-w)n_{S_0} + wn_{S_1}$; and,

$$\mathcal{E}_{\rm Hx/H/x/c}^w := (1-w)E_{{\rm Hx/H/x/c},S_0} + wE_{{\rm Hx/H/x/c},S_1} \; . \tag{S62}$$

The figure also shows the GL2 energies, for comparison.

The ISI model interpolates between correct high-density and low-density behaviours, with the former treated exactly and the latter treated using the hPC model. [18] Its use of low-density behaviours helps it to overcome major limitations of the GL2 model that is based only on low $\lambda$ behaviour only, so is unable to capture correct low-density asymptotes.

Note, for the low-density limit there is, arguably, a case to be made that it is appropriate to use $\mathcal{E}_{\rm H}$ instead of $E_{\rm H}$. This involves setting, $z = \mathcal{E}_{\rm x}^w[n^w] - W^{\rm hPC}[n^w]$ [see in the text just

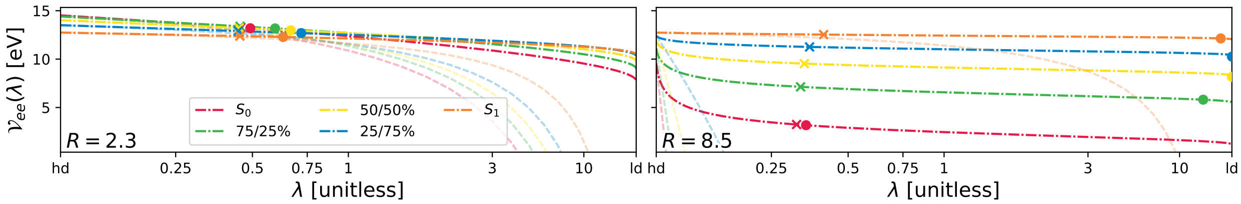


SUPPLEMENTARY FIGURE 3: Like Supplementary Figure 2 but using the ensemble Hartree in the low-density limit.

below eq. (S61)] and replacing $E_{\rm H}[n^w]$ by $\mathcal{E}_{\rm H}$ in the first term of eq. (S61). In the case of $H_2$ this makes nearly no difference to energies of $S_0$ and $S_1$, as shown in Supplementary Figure 3, but it does make mid-weighted ensembles more linear as a function of $w$ (looking vertically in the figure).

### B. Ring of quantum wells with disorder

Our second model involves model periodic physics in a minimal basis set. First, we define a geometry such that $n(x+P,y,z)=n(x,y,z)$ is on a ring. We define four "wells" at $X_{1\ldots4}$, which each have an external potential, $V_i(x,y,z)=\frac{1}{2}K[(\tilde{x}-X_i)^2+y^2+z^2]$, where $\bar{x}$ is the nearest value of $x$ to $X_i$, modulo the period, $P$. Then, the external potential is set to its value in the nearest well, giving, $v(\boldsymbol{r})=\min_{i\in 1\ldots 4}V_i(\boldsymbol{r})$. Thus, the well-depth $K$, nuclear positions $X_i$ and period $P$ are sufficient to parametrize the full system.

As a basis, we use Gaussians located at the center of each well,

$$B_p(\boldsymbol{r}) = b_p(x)\big(\tfrac{K}{\pi}\big)^{1/2}e^{-\frac{K}{2}(y^2+z^2)}\,, \qquad b_p(x)=\big(\tfrac{K}{\pi}\big)^{1/4}e^{-\frac{K}{2}|\bar{x}-X_p|^2}\,, \tag{S63}$$

where, again, we choose $\bar{x}$ closest (modulo $P$) to $X_p$. This yields overlap, kinetic energy and potential energy matrices,

$$S_{pq} = e^{-\frac{K}{4}\bar{D}_pq^2}\,, \qquad T_{pq} = \frac{K}{4}\big[3-\tfrac{KD_{pq}^2}{2}\big]S_{pq}\,, \qquad V_{pq} = \frac{K}{4}\big[2+\bar{v}_{pq}\big]S_{pq}\,, \tag{S64}$$

where $\bar{D}_{pq}=|X_p-X_q|$ is the nearest distance between $X_p$ and $X_q$ (modulo $P$); and $\bar{v}=S_{pq}^{-1}\int b_p(x)b_q(x)v(x,0,0)dx$ (with appropriate adjustments for periodicity). Finally, the electron repulsion integrals (ERI) are,

$$[pq|rs]_B = \int B_p(\boldsymbol{r})B_q(\boldsymbol{r})B_r(\boldsymbol{r}')B_s(\boldsymbol{r}')\frac{d\boldsymbol{r}d\boldsymbol{r}'}{|\boldsymbol{r}-\boldsymbol{r}'|} = S_{pq}S_{rs}\frac{\mathrm{erf}\big(\sqrt{\frac{K}{2}}D_{pq,rs}\big)}{D_{pq,rs}} \tag{S65}$$

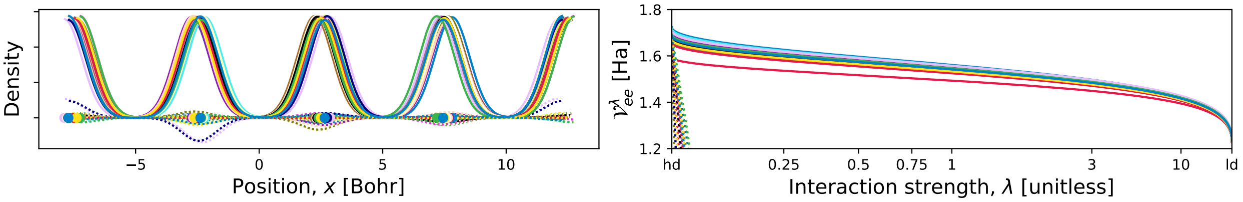


SUPPLEMENTARY FIGURE 4: **Left panel**: Densities of interacting equally weighted ensembles (solid lines) and errors in KS densities (dotted lines) for all 25 Anderson localization model runs, which reveal that both are similar in general. **Right panel**: ISI adiabatic connection model for the 25 runs (solid lines) and GL2 models (dotted lines), which reveal the importance of using low and high-density limit behaviour in models and failures in GL2. Colours identify different states.

where $D_{pq,rs}$ is the distance between the nearest (modulo $P$) means of $X_{pq} = \frac{1}{2}(\bar{X}_p + X_q)$ and $X_{rs} = \frac{1}{2}(\bar{X}_r + X_s)$. Note, this assumes that electrons only interact with their three nearest neighbours on either side.

We are thus able to carry out FCI calculations for the systems, to calculate energies, $E_K$, and wave functions, $|K\rangle$, in the minimal basis. This involves evaluating $H^{(1)}_{AB} = \langle\Phi_A|\hat{T} + \hat{V}|\Phi_B\rangle$ and $H^{(2)}_{AB} = \langle\Phi_A|\hat{V}_{ee}|\Phi_B\rangle$ by applying the Slater-Condon rules to all possible Slater determinants (SD) $\Phi_A$ of a given net spin. We then diagonalize, $H^{(1)}_{AB} + H^{(2)}_{AB}$, to find $E_K$ and coefficients, $C_{A,K}$, for $|K\rangle = \sum_A C_{A,K}|\Phi_A\rangle$.

To compute the KS system we *assume* that $v_{\text{Hxc}}(\boldsymbol{r}) \approx 0$ is zero; giving $\phi_k(\boldsymbol{r}) = \sum_p C_{pk}B_p(\boldsymbol{r})$ where $(T + V)C_k = \epsilon_k S C_k$. Under this assumption, we may also evaluate the ensemble KS system by diagonalizing, $H^{(1)}_{AB} + \eta H^{(2)}_{AB}$ for $\eta$ small and positive (we use $10^{-4}$). Focusing on the lowest singlet-singlet excitation, as in the case of $H_2$, the relevant KS states of the disordered systems are,

$$|S_{0,s}\rangle = |\phi_0^2\phi_1^2\rangle\,, \qquad |S_{2,s}\rangle = \tfrac{1}{\sqrt{2}}\left[|\phi_0^2\phi_1^{\uparrow}\phi_2^{\downarrow}\rangle - |\phi_0^2\phi_1^{\downarrow}\phi_2^{\uparrow}\rangle\right]\,, \tag{S66}$$

for use in $\mathcal{T}_s$, $\mathcal{E}_{\text{H}}$, $\mathcal{E}_{\text{x}}$, and $\mathcal{E}_{\text{c}}^{\text{GL2}}$. Note, the ordered system (ord) has an additional spatial symmetry yielding, $|S^{\text{ord}}_{0,s}\rangle = \frac{1}{\sqrt{2}}\left[|\phi_0^2\phi_1^{\uparrow}\phi_2^{\downarrow}\rangle - |\phi_0^2\phi_1^{\downarrow}\phi_2^{\uparrow}\rangle\right]$ and $|S^{\text{ord}}_{2,s}\rangle = \frac{1}{\sqrt{2}}\left[|\phi_0^2\phi_1^2\rangle + |\phi_0^2\phi_2^2\rangle\right]$. The fact that $|S^{\text{ord}}_{0,s}\rangle$ looks like $|S_{2,s}\rangle$ (i.e. that the energy seems to be reordered) is a direct consequence of symmetry-induced energy lowering.

We found (see left panel of Supplementary Figure. 4) in our calculations that the density of an equally weighted singlet-singlet ensemble, $\hat{\Gamma}_s = \frac{1}{2}|S_{0,s}\rangle\langle S_{0,s}| + \frac{1}{2}|S_{2,s}\rangle\langle S_{2,s}|$, was usually

close to the density of the corresponding interacting ensemble, $\hat{\Gamma} = \frac{1}{2}|S_0\rangle\langle S_0| + \frac{1}{2}|S_2\rangle\langle S_2|$. Thus, in all our EDFT calculations we set $w = \frac{1}{2}$ and use equations (S62) and (S61) to evaluate energies, with trivial modifications to include core electrons – the appendices of Ref. 19 provide necessary details. We thus approximate the EXX, GL2 and ISI singlet-singlet energies using,

$$\Delta E_{SS}^{\text{approx}} \approx 2\mathcal{E}^{\text{approx},w=1/2} - 2\mathcal{E}^{\text{approx},w=0} \,. \tag{S67}$$

Unlike the equally weighted ensemble, the ground state ($w = 0$) density is poorly reproduced by the KS state in about half of tested systems. We estimate the effect of bad KS densities on energies by: 1) inverting densities to obtain orbitals; 2) calculating EXX energies using non-inverted and inverted orbitals; 3) using the difference in energies to estimate errors in the high-density limit. Thus defined, the average error caused by bad KS densities has a mean of -0.14 eV and a standard deviation of 0.73 eV, which is small enough for illustrative purposes. We use FCI densities directly in $E_{\text{H}}$ and the hPC models, to avoid similar errors in the low-density limit.

Figure 2 of the main text shows results for a system with small disorder in the nuclear positions. These calculations use system parameters, $K = 1$, $X_{1\ldots4} = 5 + 0.25\delta_{1\ldots4}$, and $P = 20$, where $\delta$ is a unit Gaussian distributed random number. We compute energies from 25 runs. Figure 2 shows results from the first seven runs, as well as the mean over all 25 runs. The parameters ensure that interactions between different wells are small but strong enough to influence correlations. A model with equal spacing (i.e. with no randomness) yields $\Delta E_{SS} = 0.003$ eV. By contrast, we obtain $\Delta E_{SS} = 2.15$ eV averaged over the disordered systems, which highlights the importance of disorder-induced correlations.

Note, most *interacting* FCI states in the disordered models involve six or more SDs with weights $> 5\%$, so have strong multi-reference characteristics. Thus, KS calculation must capture complex multi-reference physics using just one SD for the KS ground state and two SD for the excitation. EXX predicts an average excitation energy of 4.40 eV, which is about twice the reference value of 2.15 eV and reflects the complete lack of correlations in EXX. GL2 predicts an extremely poor gap of 130 eV, but this value is untrustworthy due to numerical errors caused by small $\epsilon_2 - \epsilon_1$ [which appears in the denominator of the GL2 correlation energy, eq. (S58) – similar to $H_2$]. By contrast, ISI predicts a much improved (over EXX and GL2) average excitation energy of 1.89 eV.

The right panel of Supplementary Figure. 4 shows the GL2 and ISI model interpolation curve for all 25 runs, to explain the predicted energy gaps. The former illustrates how poorly GL2 performs, via its steep gradient caused by near-degeneracies in the KS eigenvalues [see eq. (S58)]. The latter highlights the importance of using both low- and high-density behaviours to capture the appropriate correlation physics, by revealing how errors in GL2 (high-density limit, $\lambda \to 0$) are quickly dampened by the strictly correlated physics (low-density limit, $\lambda \to \infty$).

---


[1] M. Lewin, Semi-classical limit of the Levy–Lieb functional in Density Functional Theory, C R Math **356**, 449 (2018).

[2] C. Cotar, G. Friesecke, and C. Klüppelberg, Smoothing of transport plans with fixed marginals and rigorous semiclassical limit of the hohenberg–kohn functional, Arch. Ration. Mech. An. **228**, 891 (2018).

[3] G. Friesecke, A. Gerolin, and P. Gori-Giorgi, The strong-interaction limit of density functional theory, arXiv preprint arXiv:2202.09760 (2022).

[4] P. Gori-Giorgi, G. Vignale, and M. Seidl, Electronic zero-point oscillations in the strong-interaction limit of density functional theory, J Chem Theory Comput **5**, 743 (2009).

[5] J. E. Harriman, Orthonormal orbitals for the representation of an arbitrary density, Phys Rev A **24**, 680 (1981).

[6] J. Grossi, Quantum fluctuations and kinetic correlation in the strongly interacting limit of density functional theory, PhD thesis (2020).

[7] P. Gori-Giorgi and M. Seidl, Density functional theory for strongly-interacting electrons: Perspectives for physics and chemistry, Phys. Chem. Chem. Phys **12**, 14405 (2010).

[8] J. Grossi, M. Seidl, P. Gori-Giorgi, and K. J. H. Giesbertz, Functional derivative of the zero-point-energy functional from the strong-interaction limit of density-functional theory, Phys Rev A **99**, 052504 (2019).

[9] D. G. A. Smith, L. A. Burns, A. C. Simmonett, R. M. Parrish, M. C. Schieber, R. Galvelis, P. Kraus, H. Kruse, R. D. Remigio, A. Alenaizan, A. M. James, S. Lehtola, J. P. Misiewicz, M. Scheurer, R. A. Shaw, J. B. Schriber, Y. Xie, Z. L. Glick, D. A. Sirianni, J. S. O'Brien, J. M. Waldrop, A. Kumar, E. G. Hohenstein, B. P. Pritchard, B. R. Brooks, H. F. Schaefer,

A. Y. Sokolov, K. Patkowski, A. E. DePrince, U. Bozkaya, R. A. King, F. A. Evangelista, J. M. Turney, T. D. Crawford, and C. D. Sherrill, Psi4 1.4: Open-source software for high-throughput quantum chemistry, J. Chem. Phys. **152**, 184108 (2020).

[10] F. Weigend and R. Ahlrichs, Balanced basis sets of split valence, triple zeta valence and quadruple zeta valence quality for H to Rn: Design and assessment of accuracy, Phys Chem Chem Phys **7**, 3297 (2005).

[11] A. Görling and M. Levy, Correlation-energy functional and its high-density limit obtained from a coupling-constant perturbation expansion, Phys Rev B **47**, 13105 (1993).

[12] T. Gould, G. Stefanucci, and S. Pittalis, Ensemble density functional theory: Insight from the fluctuation-dissipation theorem, Phys Rev Lett **125**, 233001 (2020).

[13] Z. Yang, Second-order perturbative correlation energy functional in the ensemble density-functional theory, Phys Rev A **104**, 052806 (2021).

[14] T. Gould and S. Pittalis, Hartree and exchange in ensemble density functional theory: Avoiding the nonuniqueness disaster, Phys Rev Lett **119**, 243001 (2017).

[15] T. Gould and S. Pittalis, Density-driven correlations in ensemble density functional theory: Insights from simple excitations in atoms, Aust J Chem **73**, 714 (2020).

[16] J. Lee and M. Head-Gordon, Regularized orbital-optimized second-order møller–plesset perturbation theory: A reliable fifth-order-scaling electron correlation model with orbital energy dependent regularizers, J Chem Theory Comput **14**, 5203 (2018).

[17] M. Seidl, J. P. Perdew, and S. Kurth, Density functionals for the strong-interaction limit, Phys Rev A **62**, 012502 (2000).

[18] S. Śmiga, F. D. Sala, P. Gori-Giorgi, and E. Fabiano, Self-consistent implementation of Kohn-Sham adiabatic connection models with improved treatment of the strong-interaction limit, J Chem Theory Comput 10.1021/acs.jctc.2c00352 (2022).

[19] T. Gould, L. Kronik, and S. Pittalis, Double excitations in molecules from ensemble density functionals: Theory and approximations, Phys Rev A **104**, 022803 (2021).
